# Supplementary material for: Explainability Case Studies
Source: arXiv:2009.00246 ancillary file (2020-10-03)

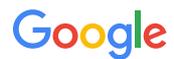

# Explainability Case Studies

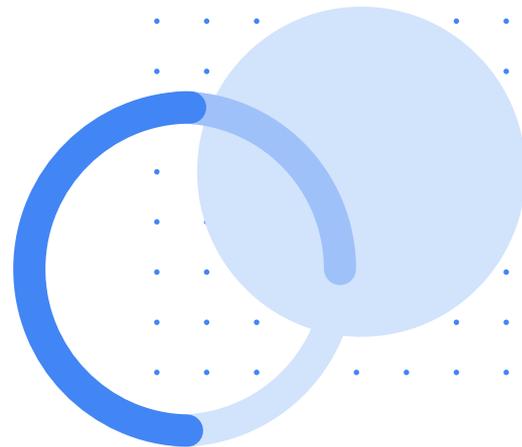

# Agenda

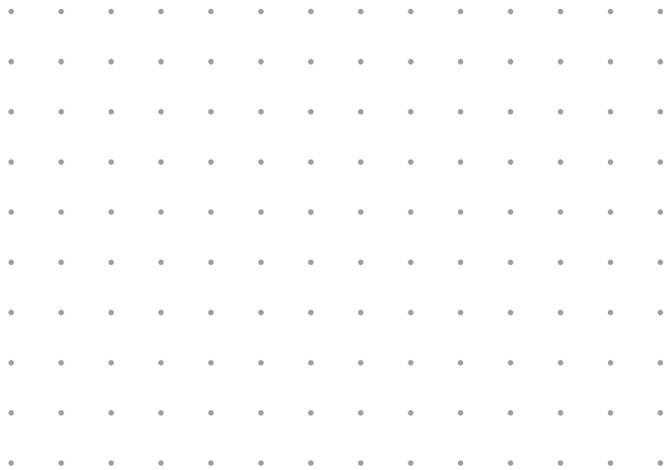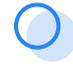

**Intro to Explainability – 15m**

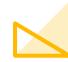

**The Model-U – 5m**

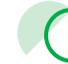

**Case Studies**

Situation 1 – 25m

Situation 2 – 20m

Situation 3 – 15m

Situation 4 – 20m

Situation 5 – 25m

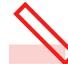

**Debrief – 25m**

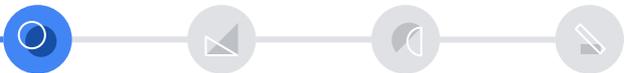

# Introductions

Your name and one answer:

- What's a **good** example of an explanation in a technology product?
- What's a **bad** example of an explanation in a technology product?
- What actually are explanations in AI systems and why are they **important** to consider in the first place?

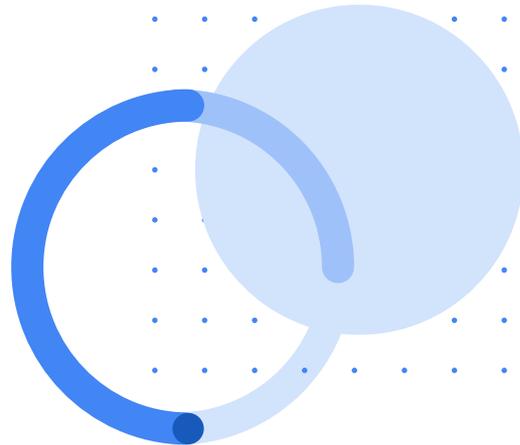

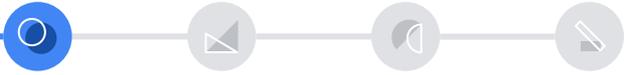

# Explainability

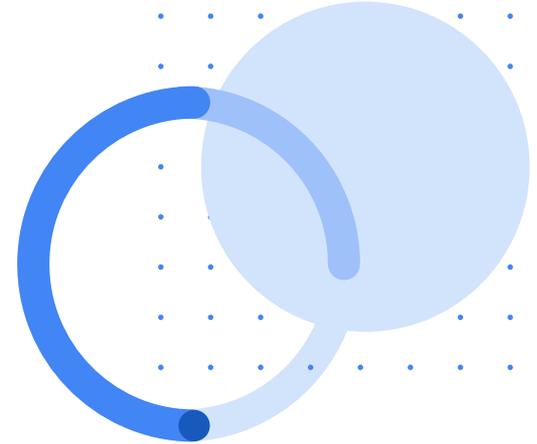

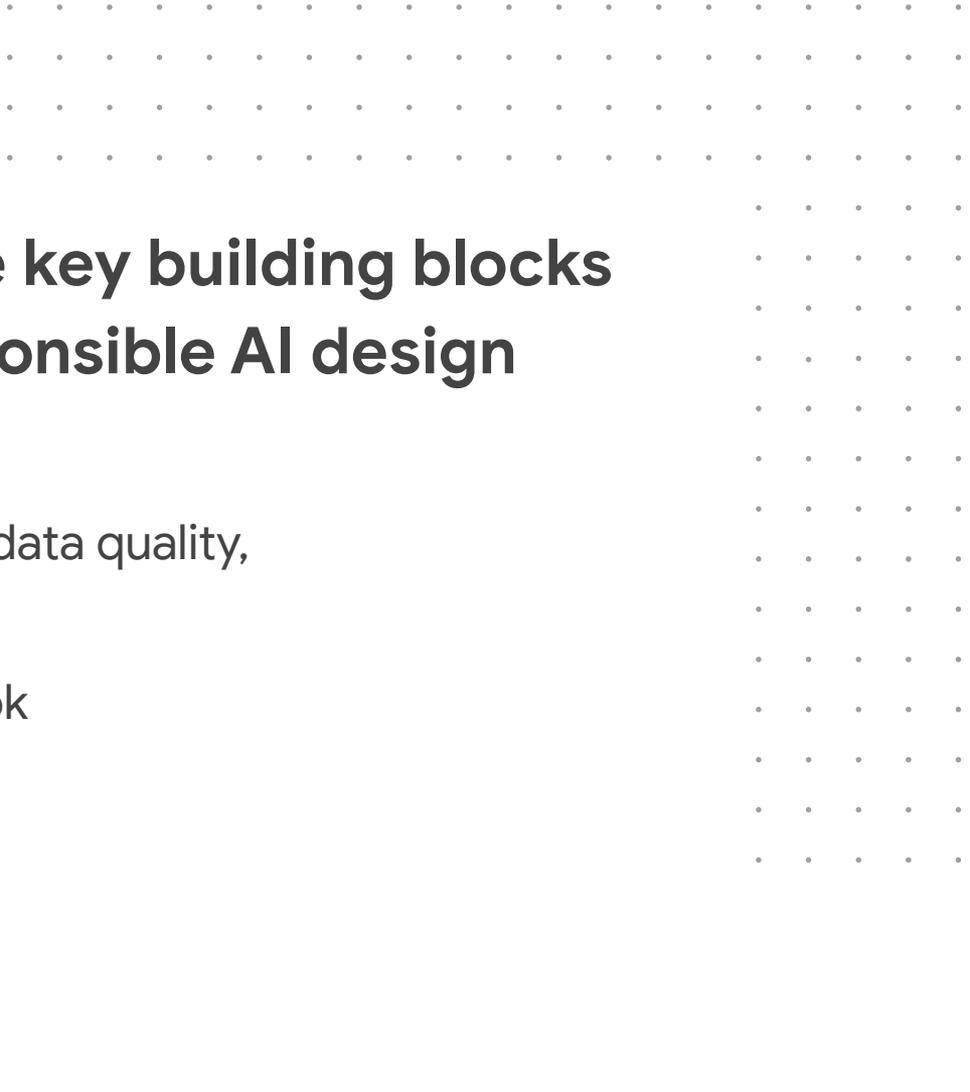

# Explainability is one of the key building blocks for human-centered, responsible AI design

along with fairness, user needs, data quality,  
feedback, control, and more...

Learn more at the Pair Guidebook

[pair.withgoogle.com/guidebook/](https://pair.withgoogle.com/guidebook/)

## DEFINITION

### **What is explainability?**

The ability to provide human understandable reasons for decisions made by an AI system

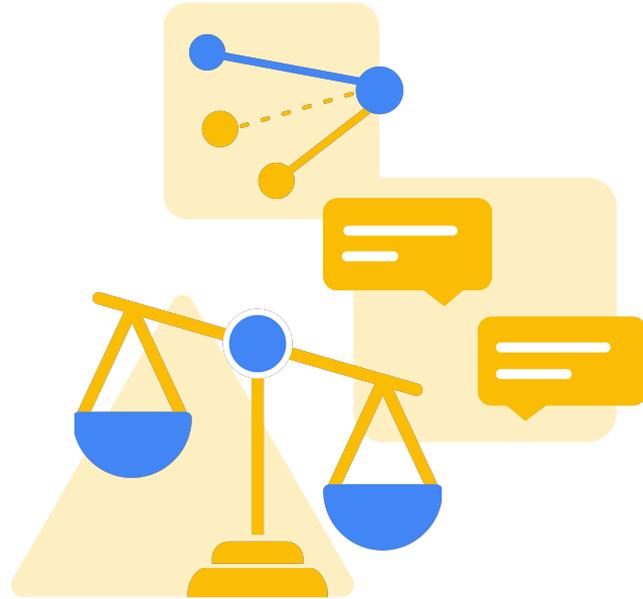

## What is explainability?

The ability to provide human understandable reasons for decisions made by an AI system

*For people to truly understand these decisions, they benefit from:*

**In-the-moment** explanations

Ongoing **education** to understand the system

An understanding of **why** a system  
has (not) changed decisions about you

Description of **consequences** and risks

Identification of potential **actions**

Results of longer-term investigation or **community engagement**

# A Broad View of Explainability

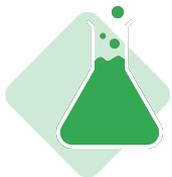

Good in-the-moment explanations

When appropriate, provide clarity for a given decision

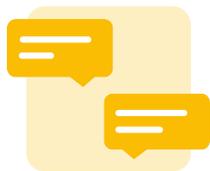

Additional explanations in product

Leverage other in-product moments where we can explain AI systems

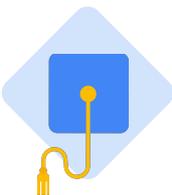

Beyond the product experience

Broaden the scope of education beyond products

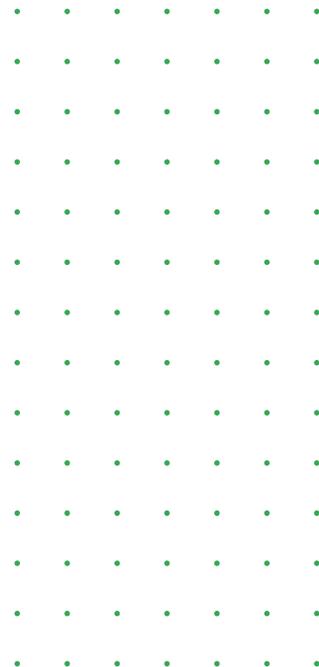

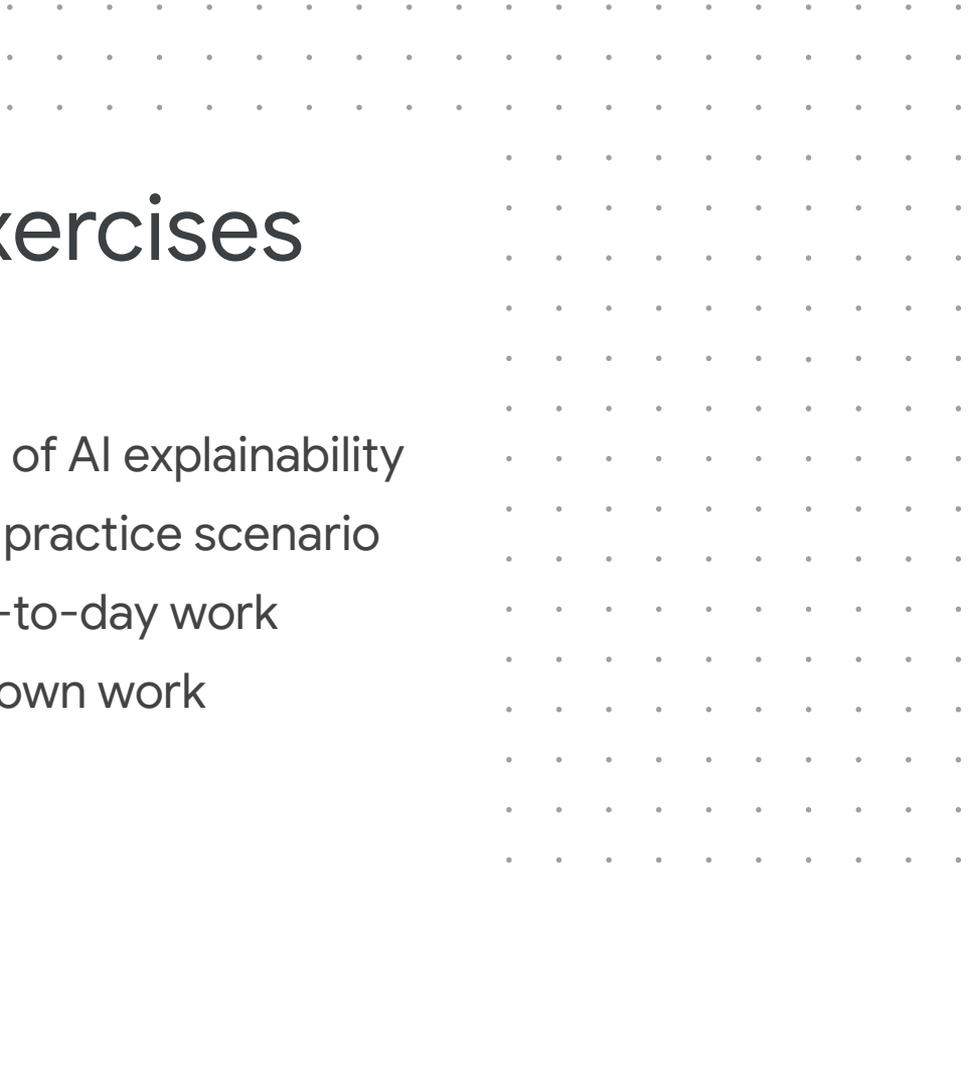

# Goals for Today's Exercises

These cases:

- will help you consider the design of AI explainability
- are not written to present a best practice scenario
- will take you outside of your day-to-day work
- should inspire new ideas in your own work

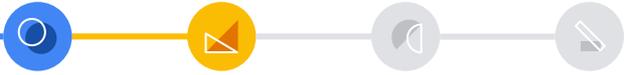

# The Model-U

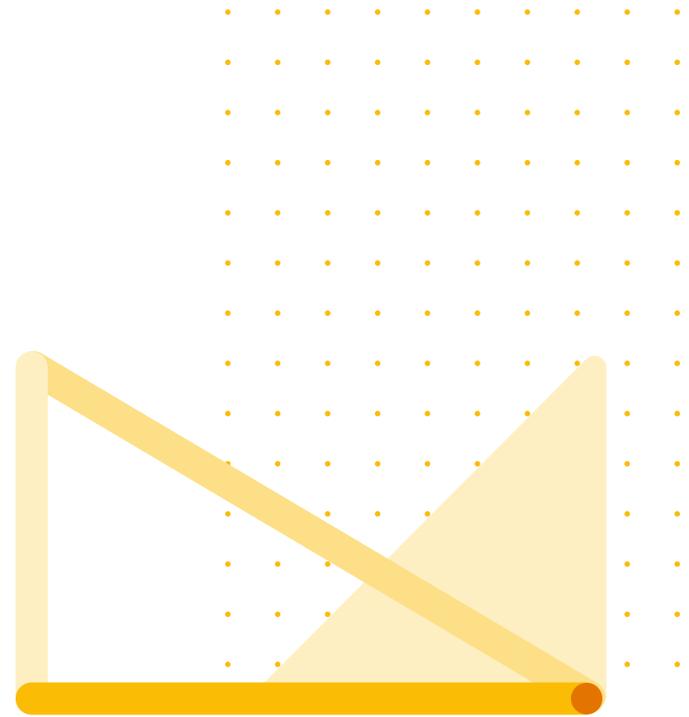

# The Model-U **overview**

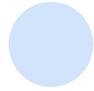

Is a **stylish car** that features a set of **integrated AI systems** that provide a revolutionary new driving experience

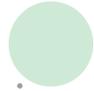

Is currently **only sold to drivers in a small part of the country**, to test its functionalities in the real world

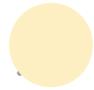

Is being **sold directly by Intelligent Engines to consumers**  
... and for this workshop we aren't going to focus on insurance & liability

# The Model-U **enhanced systems**

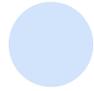

It is fitted with a variety of **audio and visual sensors** that enable a **personalized** approach by **identifying the driver and passengers**

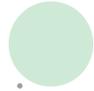

The passengers and the driver have **their own personal touchscreen**, and a state-of-the-art, **personalized entertainment system**

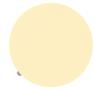

It has the **same familiar layout as today's cars** with forward-facing seats, a driving wheel, and one row of seats in the back

# The Model-U **self-driving**

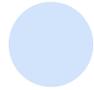

It has a **reliable self-driving capability**, and **advanced assistance in parking lots**

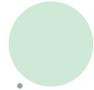

The self-driving option is so reliable that drivers can **spend their time on highways immersed in other things**, until the car nears a highway exit

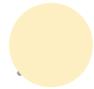

Drivers are dismayed that policy makers have **not yet given Intelligent Engines regulatory approval** to enable the self-driving feature on non-highways, even though it has been extensively tested on local roads

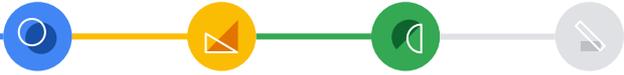

# Case studies

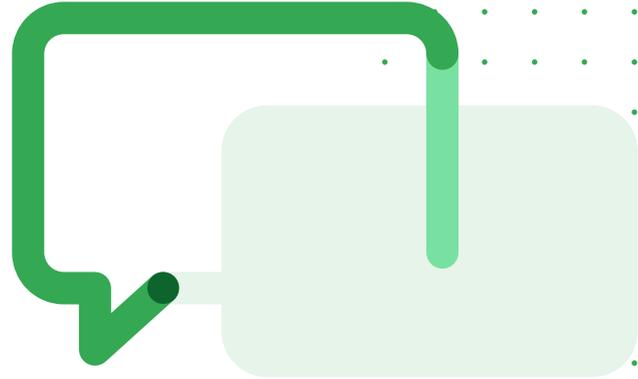

Break into groups  
and discuss

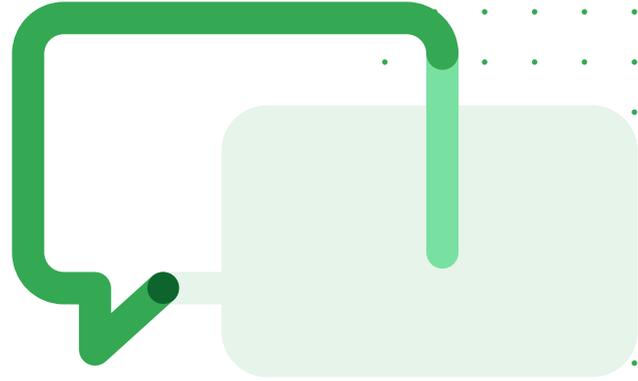

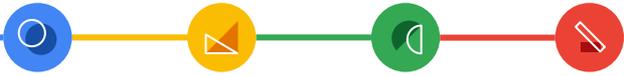

# Debrief

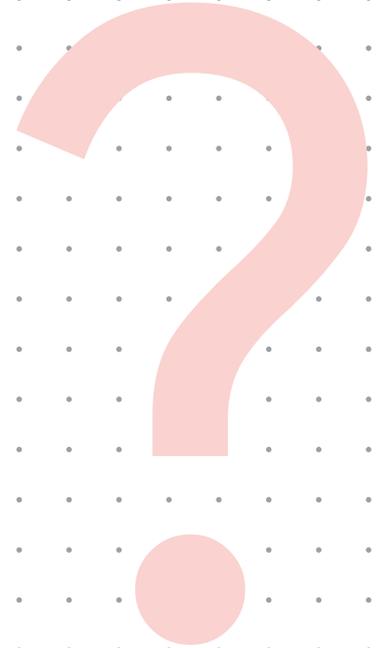

Let's all come back  
together and  
share what we  
discussed

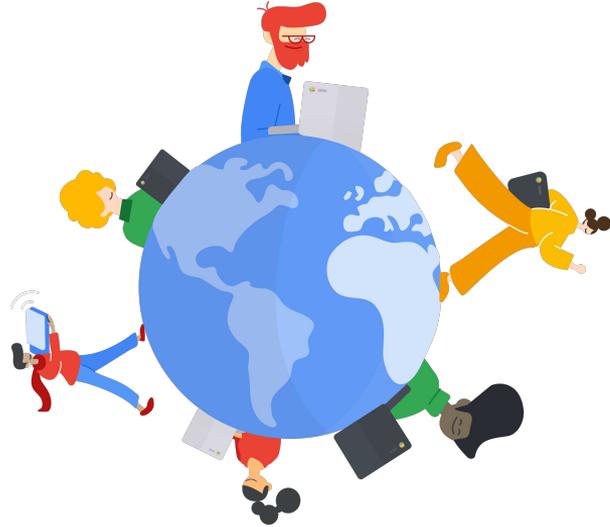

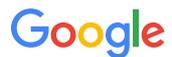

# Thanks!

This activity was developed by researchers at Google

Ben Zevenbergen, Allison Woodruff, and Patrick Gage Kelley.  
Explainability Case Studies. CSCW 2020 Workshop on Ethics in Design.

<https://arxiv.org/abs/2009.00246>

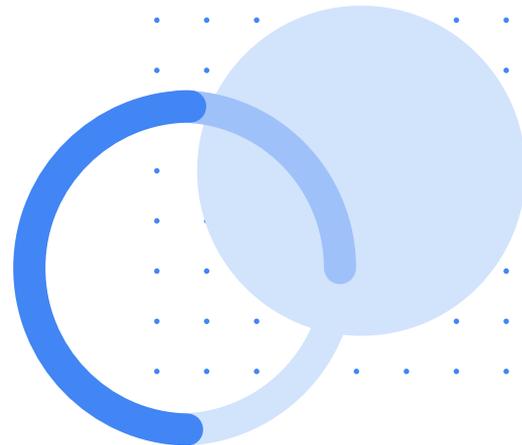

Supplement: Supplementary file 1 [file Exp-Deck.pdf]
