# Supplementary material for: Explainability Case Studies
Source: arXiv:2009.00246 ancillary file (2020-10-03)
Supplement: Supplementary file 2 [file Exp-Readme.pdf]

# Explainability Case Studies – Readme

## Table of contents

|                            |   |
|----------------------------|---|
| arXiv Entry                | 1 |
| Introduction               | 1 |
| List of materials          | 1 |
| Audience                   | 2 |
| How to use these materials | 2 |
| Timing                     | 2 |
| Situation descriptions     | 3 |
| Character introduction     | 4 |
| Sample debrief questions   | 4 |
| Citation                   | 4 |
| Contact info               | 4 |

## arXiv Entry

The full materials including this Readme can be found at <https://arxiv.org/abs/2009.00246>

## Introduction

These explainability case studies are a pedagogical tool, intended to be deliberated in an in-person or virtual workshop setting. The cases intentionally include some questionable or problematic explainability practices. In each of five situations, workshop participants discuss how and why to improve the design of the AI systems and their explanations.

This approach takes participants out of their day-to-day context and places them into hypothetical situations where an existing (though incomplete) explainability strategy is re-thought from the ground up. Using this approach, participants engage with ideas that underlie explainability best practices so they may then apply them in their own work.

The case studies are hypothetical and revolve around an imagined high tech new car—The Model-U—with audio and visual sensors for identification of passengers, a personalized entertainment system, a reliable self-driving service, including taking complete driving control on highways, and advanced assistance in parking lots. Each of these features and systems are explored in the case studies.

## List of materials

The arXiv entry contains all materials needed to run these case studies with a group of participants:

1. **Readme** (this document). The Readme provides an overview of the case studies and guidance on how to run an in-person or virtual workshop.
2. **Workshop Deck**. The slide deck contains an agenda for the activities, an introduction to the basic concepts, and an overview of the Model-U and its features.
3. **Workshop Situations**. Each of the five situations has the written case, as well as discussion prompts to help participants work through the ethics and values questions the cases describe. The table below summarizes the main themes and a short description of each situation.

# Audience

These materials are designed for audiences interested in the design and development of technology, including but not limited to practitioners, developers, user experience professionals, and undergraduate or graduate students. No specific background or expertise is required.

# How to use these materials

We have designed the workshop as follows:

- To start the workshop, you can present the Workshop Deck to introduce the activity, the concept, and the aim of the workshop.
- The Workshop Situation documents can be printed or shared virtually with participants.
- There are 5 situations, and while there is a narrative arc to the situations, you can pick and choose which you would like to cover. The table below has descriptions that can help you choose which will work best for you.
- You will likely want to break participants into groups of 3-5 to discuss the situations. If you are running the workshop virtually, you may want to have everyone rejoin the main group in between each situation to touch base, or you may want the breakout groups to work independently on multiple situations and then rejoin for a debrief.
- The materials are designed so that each group can self-moderate to work through the questions for each situation, or so that moderators can facilitate group discussion of each situation. We recommend encouraging discussion among participants, and ensuring space for all participants to share their ideas and opinions.
- If you are running the workshop virtually, you may want to create a shared notes doc for each group where participants can take notes together.
- In total, the workshop will take about 3 hours if you do all the situations and a debrief session and allow a short amount of time for breaks.

# Timing

We have found the following timing to work well, and of course recognize that you may wish to modify this to suit your specific situation.

- Introduction — 15 minutes
- The Model-U — 5 minutes
- Situation 1 — 25 minutes
- Situation 2 — 20 minutes
- Situation 3 — 15 minutes
- Situation 4 — 20 minutes
- Situation 5 — 25 minutes
- Debrief — 25 minutes

## Situation descriptions

| Scenario | Situation                                                                                                                                                                                                                                                                                                                                                                   | Themes                                                                                                                                                                                                                                |
|----------|-----------------------------------------------------------------------------------------------------------------------------------------------------------------------------------------------------------------------------------------------------------------------------------------------------------------------------------------------------------------------------|---------------------------------------------------------------------------------------------------------------------------------------------------------------------------------------------------------------------------------------|
| 1        | A family enters their newly purchased Model-U and are confronted with its identification system for the first time. One person is identified correctly and another is not, and the associated explanations cause user frustration.                                                                                                                                          | <ul style="list-style-type: none"> <li>• Superfluous content</li> <li>• Inappropriate timing</li> <li>• Explaining errors and uncertainty</li> <li>• Empowering user action</li> </ul>                                                |
| 2        | A driver merges onto the highway but is not ready to relinquish control of the Model-U to the self-driving system. The system's response makes an already complicated situation more stressful.                                                                                                                                                                             | <ul style="list-style-type: none"> <li>• Awareness of the user's context</li> <li>• Tone of explanation</li> <li>• Timeliness of content</li> <li>• Company response to user complaint about explanation</li> </ul>                   |
| 3        | The car's entertainment system recommends music, but it is unclear how user feedback informs its choices. The driver realizes they don't know enough about how the system works.                                                                                                                                                                                            | <ul style="list-style-type: none"> <li>• Providing meaningful feedback</li> <li>• Scarce attention</li> <li>• Incomplete mental models</li> <li>• Seeking appropriate moments for feedback</li> </ul>                                 |
| 4        | The Model-U is in a minor accident, and the driver receives a complex, formal explanation that is not meaningful to them. Investigation reveals the accident was caused by an adversarial attack, and the company's public response is not sufficiently reassuring.                                                                                                         | <ul style="list-style-type: none"> <li>• Varying end-user needs</li> <li>• Investigation of a high-profile failure</li> <li>• Public transparency</li> <li>• Communicating remote possibly of errors</li> </ul>                       |
| 5        | Increased ownership of Model-U's leads to congestion in towns near highways due to its traffic avoidance system. A local council organizes a stakeholder meeting which turns into a participatory design exercise. There is a tension between the information the community members want so they can co-develop policy, and what the company is willing or able to provide. | <ul style="list-style-type: none"> <li>• Community participation and feedback</li> <li>• Public information provision</li> <li>• Responsiveness to diverse information requirements</li> <li>• Limitations on transparency</li> </ul> |

## Character introduction

In the situations, we encounter a number of characters, including the following:

- Olivia and Richard recently bought a Model-U. They have two children, Timothy (an elementary schooler) and Christina (a preschooler).
- Alex and Blake are friends of Olivia and Richard.
- Sofia and Omar are technology activists.

## Sample debrief questions

1. Can you think of any technology products that give explanations at inconvenient or inappropriate times? How could those explanations be improved?
2. [*for Situation 3*] How does Richard's experience with training the entertainment system apply to how (+ if and when) you might explain to users what [PRODUCT] is doing and whether the user has any control over it?
3. [*for Situation 5*] What technology product have you seen thoughtful community discussions about?
4. [*for Situation 5*] Can you think of technology products for which it would be beneficial to provide ongoing explanations to a particular group or community?

## Citation

We suggest the following citation for these materials:

Ben Zevenbergen, Allison Woodruff, and Patrick Gage Kelley. Explainability Case Studies. CSCW 2020 Workshop on Ethics in Design. <https://arxiv.org/abs/2009.00246>

## Contact info

Please contact the authors of these case studies with any questions or comments:

- [benzevenbergen@google.com](mailto:benzevenbergen@google.com)
- [woodruff@acm.org](mailto:woodruff@acm.org)
- [patrickgage@acm.org](mailto:patrickgage@acm.org)
