# Supplementary material for: Explainability Case Studies
Source: arXiv:2009.00246 ancillary file (2020-10-03)
Supplement: Supplementary file 3 [file Exp-Situations.pdf]

# Explainability Case Studies

## Overview

These case studies cover 5 hypothetical situations, which intentionally include some questionable or problematic explainability practices. For each situation, workshop participants can discuss how and why to improve the design of the AI systems and their explanations.

## Introducing the car

The case studies revolve around an imagined high tech new car—The Model-U—with audio and visual sensors for identification of passengers, a personalized entertainment system, a reliable self-driving service, including taking complete driving control on highways, and advanced assistance in parking lots. The Model-U is sold directly by Intelligent Engines to consumers, but currently it is only sold to drivers in a small part of the country, to test its functionalities in the real world. The self-driving option is so reliable that drivers can spend their time on highways immersed in other things, until the car nears a highway exit. Drivers are dismayed that policy makers have not yet given Intelligent Engines regulatory approval to enable the self-driving feature on non-highways, even though it has been extensively tested on local roads.

## Introducing the characters

In the situations, you will encounter a number of characters, including the following:

- Olivia and Richard recently bought a Model-U. They have two children, Timothy (an elementary schooler) and Christina (a preschooler).
- Alex and Blake are friends of Olivia and Richard.
- Sofia and Omar are technology activists.

## Citation

We suggest the following citation for these materials:

Ben Zevenbergen, Allison Woodruff, and Patrick Gage Kelley. Explainability Case Studies. CSCW 2020 Workshop on Ethics in Design. <https://arxiv.org/abs/2009.00246>



## Situation 1: Identification and tailored service

Olivia and Richard recently bought their first Model-U to improve the comfort of their commutes and to enhance family activities while on the road. Their first trip is to visit family friends who live a few hours' drive away in a beautiful small town outside of the metropolitan area. The couple enter the new car with their children Timothy (an elementary schooler) and Christina (a preschooler). The family is very excited to experience the futuristic features the car has to offer for the first time. Upon entering, a friendly automated voice asks:

"How are you today?"

Olivia, who had rushed to the driving seat ahead of Richard, responds excitedly. The Model-U confirms:

"Can I confirm that Olivia will be driving today?"

Amazed that the car identified her correctly as sitting in the driving seat, Olivia exclaims "Yes! I am!" The Model-U identifies and authenticates drivers by triangulating the biometric voice profile with the facial features of the driver. This process begins when owners purchase the car, at which point they download an app. Each individual registered driver has to agree to the Model-U's terms of service and privacy policy documents by saying "Yes, I have read and agreed to the documents" out loud to the app, which establishes their voice profile. When they first enter the car, each registered driver types in a security pincode (provided by the app) and must sit in the driving seat to have a 3-D biometric profile of their face be compiled by the car.

The Model-U team went out of their way to be good stewards of their biometric identification system by making known the existence of the system, the technologies and logic of the identification, as well as explaining possible consequences. After confirming Olivia, the Model-U provides the following explanation of the procedure:

"Welcome back to your Model-U Olivia! I have determined with a 93% certainty that Olivia is the person sitting behind the wheel by analysing the biometric data taken from the dashboard camera, which was trained on a nationally-representative dataset. To further verify the accuracy of the driver's identity to the required threshold level of 99.9%, I used the matched voiceprint. The collection of data is a processing of your personal data or personally identifiable information according to applicable laws. The Model-U uses your personal data to provide you with a better experience. For example, your confirmed identity allows you to start the car's engine. Your personal data will be used to tailor the entertainment experience for you. And in the unlikely case of a collision, we will be able to determine to whom we send an automated accident report."

### Questions 1A

1. List a few pieces of information in this explanation.
2. What information on your list is meaningful, appropriate, and timely for a driver who has just entered the car for the first time?
3. What information on your list is useful every time the driver gets into the car?
4. Do you think this is a good explanation? Why or why not?

After a pleasurable first journey, the family arrives at their friends' Alex and Blake's house. Blake has been eagerly awaiting the arrival of their friends, mostly because he wanted to try out the Model-U. After some friendly greetings, Olivia allows Blake to take a seat behind the wheel. To their initial surprise, the friendly voice says:

"I'm sorry, I was not able to identify the driver. Please adjust your face for the camera."

Olivia and Richard realize quickly that of course it didn't recognize Blake, since he'd never been registered. Richard asks to take Blake's place in the car just to get the system started, so Blake could experience the various services and apps for himself. To his surprise, with Richard in the driver's seat the car repeats the same apology:

"I'm sorry, I was not able to identify the driver. Please adjust your face for the camera."

Richard takes off his sunglasses and faces the camera on the steering wheel, only to hear the same apology once again. Every attempt to realign his face to the camera fails. He checks the Model-U app and confirms it had, indeed, created and stored a facial profile. Richard finally presses the 'Help' button on the screen, which provides the following explanation:

"I could not identify the driver at the required threshold level of certainty. There may be several reasons for this, including a change in facial features since your profile was created, an inaccurate profile was created, or a faulty camera. Further, the cameras in the car may be malfunctioning or be partially blocked, thereby distorting the image. You may enter the 8-digit pin code you were provided to start the Model-U."

### Questions 1B

1. Are these good explanations of the identification failures? If not, why not?
2. Discuss some approaches for more helpful explanations.
3. In situations where the Model-U does not successfully identify a registered driver, what mechanism should be provided so they can start their car and how should it be communicated to them?

## Situation 2: Highway detection

After an enjoyable day, Olivia, Richard, Timothy, and Christina get back in the car as soon as daylight fades and the evening's clouds begin to form. Olivia takes the wheel again, eager to continue trying out more new features of the Model-U. On their return journey, the family decides to use the nearby highway, which is typically less busy in the evenings.

As Olivia enters the acceleration lane of the highway, the friendly automated voice asks whether she is willing to relinquish control to the Model-U's systems.

"I have detected you're about to merge onto a highway. Do you want the Model-U to take over driving for you now?"

Anxiety creeps up on Olivia. When she sees their two children in the back of the car through their rearview mirror, she suddenly has a change of heart. Olivia doesn't want to subject their whole family to this first experiment with the new self-driving technology. She responds "no" and tells Richard she'd rather test the functionality by herself first. When Richard attempts to respond to Olivia, their conversation is cut short by an unexpected explanation from the system, which states:

"I recommend you allow the Model-U to drive on this highway. I have calculated a higher than normal danger rating and an increased risk of collisions by human-operated cars in these conditions. This is based on the amount of cars on the highway, the reduced visibility, and the time of day. The risk of collisions is significantly higher for this journey. Your car insurance will not cover the full amount of your Model-U insurance in case of an accident when you control the car. Do you wish to reconsider the self-driving option now?"

Olivia's anxiety increases further. Puzzled, Richard and Olivia look at each other. Timothy nervously asks his parents what the voice is saying. Olivia does not have an immediate response to anyone and tries to focus on driving on the highway. The friendly voice repeats the question whether it should take over the driving, but Olivia just feels overwhelmed. The warning of an increased risk doesn't mean anything to her, as she never previously witnessed a collision on this particular highway. Upon their arrival at home, Olivia files a complaint with Intelligent Engines about this lengthy and complicated explanation.

### Questions 2

1. Is the explanation a good fit for the driver's situation? Why or why not?
2. What information does Olivia need at the moment she considers the self-driving option, and why?
3. Which information could be provided to Olivia at a different time instead, and how could it be presented to her?
4. How should Intelligent Engines respond to Olivia, and what actions should it take based on her complaint?

## Situation 3: Entertainment recommender system

As a family routine, Olivia and Richard bring their children to school as part of their commute in the mornings. Model-U successfully identifies Richard as the driver and presents him with a list of audio options ranging from his favorite artists, kids music playlists, audiobooks, and news updates. Instead of choosing a particular option, he just presses the PLAY button to have the Model-U select music. He is pleased when all options disappear from the dashboard and are replaced by this logo:

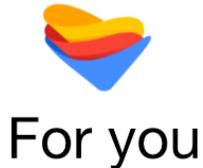

When the logo lights up, the family hears the following audio message:

"I will now select music relevant to you. Please let me know whether I'm getting your preferences right"

On their way to school, the family discuss the day ahead while listening to the music chosen by the Model-U. Near the end of each song, Richard asks his children what they thought of the song. If and when the children agree that a song was good, Richard touches the thumbs up button on the right of the steering wheel. When the democratic vote is negative, Richard presses the thumbs down button on the left. After a few songs, the car says:

"Thank you for your feedback, Richard. We're using your expressed preferences to improve the model and tailor the selection to your taste"

Suddenly, Richard realizes that he is unsure to which profile he was contributing ratings. Who does the 'You' in the logo refer to, he wonders. He begins to worry that he may have been contributing ratings of children's music to his own entertainment profile, so the Model-U may continue to play children's music when he is driving the car without his kids. When he asks the Model-U to revert the ratings given in the current journey, the car responds:

"I'm sorry, I did not understand your command. Did you wish to review your music history?"

While this is not exactly what Richard wanted, he is intrigued whether he could manipulate his music history and previous feedback to influence any future recommendations. However, he realizes he shouldn't review his personal history while driving a car and says "No." He would, however, like to do that later to understand better how the Model-U's music recommendation system works.

### Questions 3

1. If Richard answers "Yes", how should the music review feature work since he is driving?
2. How should the music review feature work when the user is not driving?
3. Does Richard understand enough about how the entertainment recommender system chooses songs? If not, what does he need to learn in order to meaningfully influence it?

## Situation 4: Accident investigation

As Olivia and Richard spend more time in their car, they begin to notice some quirks and inconsistencies in its behavior. For example, the self-parking feature works well most of the time, allowing the car to squeeze into small spaces by performing parallel parking to an expert level. Sometimes, though, the car may jolt, swerve slightly off course, and reattempt a parking maneuver for no discernible reason.

Olivia's and Richard's enthusiasm for their new car is challenged when the Model-U causes minor scratches on theirs and another person's car. In an overly full parking lot, Olivia had commanded the car to find a spot and park automatically. When the Model-U began its slow reverse maneuver into one of the last remaining empty spots and Olivia was getting her possessions ready, she noticed that the car stopped suddenly. It then moved forwards and backwards a few times, and she eventually heard a scratching noise. Immediately, the following notification is displayed on the dashboard:

Minor collision detected. Please touch this screen to generate an accident report.

She decides to get out of the car to inspect what happened. Upon examination, Olivia notes that the other car is parked slightly over the dividing line, though that there was ample space for the Model-U to park. She decides to stick a note with her phone number and email address under the windshield wiper of the other car. While staying calm, she is concerned that the car she placed her trust in made such a rookie parking mistake.

Shortly after touching the screen, she receives an email from Intelligent Engines that includes the accident report in an attached PDF file. However, when she opens the document, she realizes that she understands less than half of the language included in the report. Most of the documentation includes graphs that resemble statistics and rows of numbers, and includes various links to online portals that she has no access to. Discouraged, she decides to contact Intelligent Engines's customer service department, hoping to receive a better explanation. The customer service representative explains that she should present the report to her insurance company, who have the expertise in-house to make sense of the report and determine whether she and the other driver can be compensated for the damage.

Olivia posts an angry message on a social media platform where she describes the unnecessary accident and the incomprehensible automated report. To her surprise, dozens of people respond to her and describe similar experiences. The resulting discussion is picked up by a technology journalist, who publishes an article about the scratches and minor fender benders caused by Intelligent Engines's Model-U, along with the incomprehensible explanations provided to drivers by Intelligent Engines.

The Model-U team picks up on the commotion and decides to launch an investigation. The parking issues as described did not surface during the ongoing testing of the Model-U. Some members of the team have long argued that users need a better explanation than the reports that are generated for insurance purposes, and the team considers possible changes.

#### Questions 4A

1. How should a minor accident be explained to both drivers and their insurance companies?
2. At this point in time, what responsibility does the company have to investigate and act on the concerns raised on social media?
3. What information should Intelligent Engines share publicly about how they are handling the situation?

The investigation uncovers a targeted and malicious plot against the Model-U. In every automated accident report during parking maneuvers, the Model-U experienced an anomaly where an object rapidly appeared and disappeared in the parking spot. When reviewing the visual data, the team noticed a series of stickers on the ground that confused the car's computer vision algorithms with the impression that the car had to turn in one direction. However, in each case, the actual parking spots were obviously empty to the human observer of the images.

The existence of the stickers was confirmed upon closer inspection of some of the actual parking spots. They were white and contained a URL in small red letters. When the team visits the advertised website, they're presented with a lengthy blog post written by technology activists Sofia and Omar, titled 'Deceiving the Model-U with Printable Stickers'. The paper describes how the stickers, when placed in a particular order, deceive the Model-U's systems to stray from its intended path. The paper ends with a stern warning that these stickers also deceive the car when driving on a road. Their stunt had been to gain publicity for their uncovered attack vector and that they hoped to save lives.

Intelligent Engines' Model-U team decides to audit their product for further adversarial attacks. The Intelligent Engines developer relations representative publicly asks other researchers and activists to submit their uncovered adversarial attacks to their bug bounty program, rather than causing more accidents.

#### Questions 4B

1. Many AI systems can be vulnerable to adversarial attacks, even if their foreseeable likelihood is small enough to pass regulatory scrutiny. How can a remote chance of being subjected to a malicious and adversarial attack by third parties be explained to the owners or prospective buyers of the Model-U?
2. What should the team explore in their audit? What information from the audit should they explain in an external facing audit report?

## Situation 5: Rural Town

Local policy makers embrace the Model-U's routing feature that causes a reduction of traffic on major transportation arteries. When the mapping and routing algorithms find that a particular highway is close to being jammed, the Model-U suggests some alternate routes to its drivers. Typically, these alternate routes are composed of a series of roads through smaller towns and villages that happen to be near the clogged up highways. The distance may be longer, but the time traveled is calculated to be shorter than joining a traffic jam on a highway.

Local policymakers had expressly disallowed any autonomous driving beyond highways, in part because they did not trust the safety assurances provided by Intelligent Engines. Not only are there now more cars on the roads, the drivers are unfamiliar with these towns and therefore drive more slowly. Alex and Blake feel increasingly burdened by the influx of a high number of Model-U's in their town. The roads were already busy in the mornings with parents taking their children to school and commuters trying to get to work on time. Now, new and longer traffic jams are increasingly forming in villages and small towns that are not planned or designed to cope with this increased volume of traffic.

After some political debate among policymakers from a variety of counties, a joint decision was made to accommodate the self-driving features of the Model-U by "embracing though limitation". In addition to allowing self-driving cars on the roads, the proposed policy suggests to let towns and villages designate specific roads on which Model-U's may not drive autonomously when diverted from the highway. However, the policymakers stress that the locals should be able to collectively decide which roads are designated as off-limits to autonomous driving. They invite Intelligent Engines to provide information about the extent to which their plans are feasible.

Several towns and villages in the region organize stakeholder hearings where the plans, their technical feasibility, and its overall desirability are presented and discussed. Locals are invited to join the discussion and to present their points of view. Intelligent Engines decides to dispatch a few employees from its 'developer relations' team to some of the local meetings that are happening around the country, including to Alex and Blake's town. Upon hearing the presence of a company representative attending, Sofia and Omar decide to join this particular meeting, too. As owners of a Model-U who will be directly impacted, Olivia and Richard, too, attend the meeting, because no meetings are planned near their urban dwellings.

### Question 5A

1. Choose one character per participant and discuss (1) which data or information you may need to support your positions or concerns, and (2) which data or information is likely to be most meaningful in making a decision about which roads the Model-U can drive on?

| <b>Characters</b>                                                                                                                                                                                                                                                                                                                       |                                                                                                                                                                                                                                                                                                                                   |
|-----------------------------------------------------------------------------------------------------------------------------------------------------------------------------------------------------------------------------------------------------------------------------------------------------------------------------------------|-----------------------------------------------------------------------------------------------------------------------------------------------------------------------------------------------------------------------------------------------------------------------------------------------------------------------------------|
| <p><b>Olivia, Richard (Owner)</b></p> <ul style="list-style-type: none"> <li>Concerned about undue restrictions on the use of their Model-U</li> <li>Feel that autonomous driving feature is safer than human drivers</li> </ul>                                                                                                        | <p><b>Alex, Blake (Locals)</b></p> <ul style="list-style-type: none"> <li>Oppose the policy to begin with, because they don't want autonomous robots in their environment</li> <li>Concerned about general congestion in the town</li> <li>Concerned about safety on roads near schools</li> </ul>                                |
| <p><b>Sofia, Omar (Activist researchers)</b></p> <ul style="list-style-type: none"> <li>Concerned about physical safety in general</li> <li>Want to hold big corporations accountable</li> <li>Want know more about error rates and unintended negative consequences</li> <li>Want to query the Model-U's various algorithms</li> </ul> | <p><b>Local council transportation officer, local elected official</b></p> <ul style="list-style-type: none"> <li>Concerned about congestion because of policy targets and re-election</li> <li>Do not want to be seen to put corporate interests over citizens interests</li> <li>Appreciate safety claims by company</li> </ul> |

**Question 5B**

- From the point of view of Intelligent Engines, which information requested by community members in the previous question can Intelligent Engines provide? Are there any limitations that make it difficult or undesirable for a corporation to provide this information?

The first town hall meeting is a confusing affair, though a compromise is reached about the information Intelligent Engines provides to stakeholder meetings to support a fruitful participatory design exercise. The company creates maps of each region and marks the roads that are most frequently used by Model-U's navigating autonomously, without sharing any of the underlying code or other proprietary information. These maps can be used by stakeholders to discuss the desirability of blocking particular roads.

The outcome of the new "embracing through limitation" policy appeared—at first—to be a success. After several months, however, after even more Model-U's were produced and sold, some local policy makers feel it is time to evaluate the success factors and continued appropriateness of their policy. They collectively ask Intelligent Engines to provide further data and regular updates, which they cannot collect themselves but require to make an informed policy decision.

**Question 5C**

- What would the community (and especially your character) need to know on an ongoing basis to evaluate the effectiveness of the policy about which roads the Model-U can drive on?
